# Supplementary material for: ID-Patch: Robust ID Association for Group Photo Personalization
Source: arXiv:2411.13632 source file (2025-03-29)
Supplement: Supplementary file 1 [file 6_appendix.tex]

\setcounter{section}{0}

\section*{Appendix}

\setcounter{section}{0}
\setcounter{figure}{0}
\makeatletter 
% Figure counter representation
% Hyperref figure hyperlink hook

% \renewcommand{\thefigure}{A\@arabic\c@figure}
\makeatother
\setcounter{table}{0}

\setcounter{mylemma}{0}

\setcounter{equation}{0}
